# Supplementary material for: Unified Graph Networks (UGN): A Deep Neural Framework for Solving Graph Problems
Source: arXiv:2502.07500 source file (2025-02-11)
Supplement: Supplementary file 1 [file appendix_tab.tex]

\begin{table}[H]
\setlength{\tabcolsep}{5pt}
\subcaptionbox{IoT--20 node classification}{
\begin{subtable}{0.5\textwidth}
\centering
\begin{tabular}{|c|c|c|c|c|}
\hline
 & precision & recall & f1-score & support \\
\hline\hline
malicious & 0.86 & 0.43 & 0.57 & 693  \\
benevolent & 0.93 & 0.99 & 0.96 & 5,167 \\
\hline\hline
accuracy & & & 0.92 & 5,860\\
macro avg & 0.90 & 0.71 & 0.76 & 5,860 \\
weighted avg & 0.92 & 0.92 & 0.91 & 5,860 \\
\hline
\end{tabular}
\end{subtable}}
\subcaptionbox{IoT--20 edge classification}{
\begin{subtable}{0.5\textwidth}
\centering
\begin{tabular}{|c|c|c|c|c|}
\hline
 & precision & recall & f1-score & support \\
\hline\hline
Pos. Edge & 0.86 & 0.98 & 0.92 & 43,612  \\
Neg. Edge & 0.99 & 0.90 & 0.94 & 67,728 \\
\hline\hline
accuracy & & & 0.93 & 111,340\\
macro avg & 0.92 & 0.94 & 0.93 & 111,340 \\
weighted avg & 0.94 & 0.93 & 0.93 & 111,340 \\
\hline
\end{tabular}
\end{subtable}}
\subcaptionbox{IoT--40 node classification}{
\begin{subtable}{0.5\textwidth}
\centering
\begin{tabular}{|c|c|c|c|c|}
\hline
 & precision & recall & f1-score & support \\
\hline\hline
malicious & 0.90 & 0.58 & 0.70 & 1,371  \\
benevolent & 0.95 & 0.99 & 0.97 & 10,349 \\
\hline\hline
accuracy & & & 0.94 & 11,720\\
macro avg & 0.92 & 0.78 & 0.83 & 11,720 \\
weighted avg & 0.94 & 0.94 & 0.94 & 11,720 \\
\hline
\end{tabular}
\end{subtable}}
\subcaptionbox{IoT--40 edge classification}{
\begin{subtable}{0.5\textwidth}
\centering
\begin{tabular}{|c|c|c|c|c|}
\hline
 & precision & recall & f1-score & support \\
\hline\hline
Pos. Edge & 0.89 & 0.98 & 0.93 & 131,558  \\
Neg. Edge & 0.99 & 0.95 & 0.97 & 325,522 \\
\hline\hline
accuracy & & & 0.96 & 457,080 \\
macro avg & 0.94 & 0.97 & 0.95 & 457,080 \\
weighted avg & 0.96 & 0.96 & 0.96 & 457,080 \\
\hline
\end{tabular}
\end{subtable}}
\subcaptionbox{IoT--60 node classification}{
\begin{subtable}{0.5\textwidth}
\centering
\begin{tabular}{|c|c|c|c|c|}
\hline
 & precision & recall & f1-score & support \\
\hline\hline
malicious & 0.89 & 0.58 & 0.71 & 2,198  \\
benevolent & 0.94 & 0.99 & 0.97 & 15,382 \\
\hline\hline
accuracy & & & 0.94 & 17,580 \\
macro avg & 0.92 & 0.79 & 0.84 & 17,580 \\
weighted avg & 0.94 & 0.94 & 0.93 & 17,580 \\
\hline
\end{tabular}
\end{subtable}}
\subcaptionbox{IoT--60 edge classification}{
\begin{subtable}{0.5\textwidth}
\centering
\begin{tabular}{|c|c|c|c|c|}
\hline
 & precision & recall & f1-score & support \\
\hline\hline
Pos. Edge & 0.90 & 0.98 & 0.94 & 167,020  \\
Neg. Edge & 1.00 & 0.98 & 0.99 & 870,200 \\
\hline\hline
accuracy & & & 0.98 & 1,037,220 \\
macro avg & 0.95 & 0.98 & 0.96 & 1,037,220 \\
weighted avg & 0.98 & 0.98 & 0.98 & 1,037,220 \\
\hline
\end{tabular}
\end{subtable}}
\caption{Model performance on the IoT dataset}
\label{tab:IoT_PRF}
\end{table}
\begin{table}[H]
\centering
\begin{tabular}{|c|c|c|c|c|}
\hline
 & precision & recall & f1-score & support \\ [0.5ex]
\hline\hline
no bond & 0.99 & 0.99 & 0.99 & 1,543,500  \\
single bond & 0.87 & 0.89 & 0.88 & 95,902 \\
double bond & 0.71 & 0.81 & 0.76 & 14,664 \\
triple bond & 0.62 & 0.94 & 0.75 & 1,294 \\
aromatic bond & 1.00 & 1.00 & 1.00 & 68,834 \\
\hline\hline
accuracy & & & 0.98 & 1,724,194 \\
macro avg & 0.84 & 0.93 & 0.87 & 1,724,194 \\
weighted avg & 0.98 & 0.98 & 0.98 & 1,724,194 \\
\hline
micro avg of Pos. Edges & 0.90 & 0.93 & 0.91 & 180,694 \\
macro avg of Pos. Edges & 0.80 & 0.91 & 0.85 & 180,694 \\
weighted avg of Pos. Edges & 0.90 & 0.93 & 0.91 & 180,694 \\ [0.5ex]
\hline
\end{tabular}
\caption{Model Performance on the Chemistry Reaction dataset}
\label{tab:Chem_PRF}
\end{table}
\begin{table}[H]
\setlength{\tabcolsep}{5pt}
\parbox{.5\linewidth}{
\centering
\begin{tabular}{|c|c|c|c|c|}
\hline
 & precision & recall & f1-score & support \\ [0.5ex]
\hline\hline
trust & 0.80 & 0.84 & 0.82 & 100,000  \\
neg. edge & 0.84 & 0.79 & 0.81 & 100,000 \\
\hline\hline
accuracy & & & 0.82 & 200,000 \\
macro avg & 0.82 & 0.82 & 0.82 & 200,000 \\
weighted avg & 0.82 & 0.82 & 0.82 & 200,000 \\ [0.5ex]
\hline
\end{tabular}
\caption{Model Performance on the Epinions dataset}
\label{tab:Epinions_PRF}
}
\hfill
\parbox{.5\linewidth}{
\centering
\begin{tabular}{|c|c|c|c|c|}
\hline
 & precision & recall & f1-score & support \\ [0.5ex]
\hline\hline
friendship & 0.80 & 0.84 & 0.82 & 200,000  \\
neg. edge & 0.83 & 0.79 & 0.81 & 200,000 \\
\hline\hline
accuracy & & & 0.82 & 400,000 \\
macro avg & 0.82 & 0.82 & 0.82 & 400,000 \\
weighted avg & 0.82 & 0.82 & 0.82 & 400,000 \\ [0.5ex]
\hline
\end{tabular}
\caption{Model Performance on the Slashdot dataset}
\label{tab:Slashdot_PRF}
}
\end{table}
\begin{table}[H]
\setlength{\tabcolsep}{5pt}
\parbox{.5\linewidth}{
\centering
\begin{tabular}{|c|c|c|c|c|}
\hline
 & precision & recall & f1-score & support \\
\hline\hline
Community$_0$ & 1.00 & 1.00 & 1.00 & 16  \\
Community$_1$ & 1.00 & 1.00 & 1.00 & 16 \\
\hline\hline
accuracy & & & 1.00 & 32 \\
macro avg & 1.00 & 1.00 & 1.00 & 32 \\
weighted avg & 1.00 & 1.00 & 1.00 & 32 \\
\hline
\end{tabular}
\caption{Model Performance on the Zachary's karate club dataset with 2 communities}
\label{tab:karate2_PRF}
}
\hfill
\parbox{.5\linewidth}{
\centering
\begin{tabular}{|c|c|c|c|c|}
\hline
 & precision & recall & f1-score & support \\
\hline\hline
Community$_0$ & 0.92 & 0.92 & 0.92 & 12  \\
Community$_1$ & 1.00 & 0.91 & 0.95 & 11 \\
Community$_2$ & 0.75 & 1.00 & 0.86 & 3 \\
Community$_3$ & 1.00 & 1.00 & 1.00 & 4 \\
\hline\hline
accuracy & & & 0.93 & 30 \\
macro avg & 0.92 & 0.96 & 0.93 & 30 \\
weighted avg & 0.94 & 0.93 & 0.93 & 30 \\
\hline
\end{tabular}
\caption{Model Performance on the Zachary's karate club dataset with 4 communities}
\label{tab:karate4_PRF}
}
\end{table}
\begin{table}[H]
\setlength{\tabcolsep}{5pt}
\parbox{.5\linewidth}{
\centering
\begin{tabular}{|c|c|c|c|c|}
\hline
 & precision & recall & f1-score & support \\
\hline\hline
Community$_0$ & 1.00 & 1.00 & 1.00 & 8  \\
Community$_1$ & 1.00 & 1.00 & 1.00 & 7 \\
Community$_2$ & 0.91 & 1.00 & 0.95 & 10 \\
Community$_3$ & 0.92 & 1.00 & 0.96 & 11 \\
Community$_4$ & 1.00 & 0.89 & 0.94 & 9 \\
Community$_5$ & 1.00 & 0.25 & 0.40 & 4 \\
Community$_6$ & 0.86 & 1.00 & 0.92 & 12 \\
Community$_7$ & 1.00 & 1.00 & 1.00 & 7 \\
Community$_8$ & 1.00 & 1.00 & 1.00 & 9 \\
Community$_9$ & 0.92 & 1.00 & 0.96 & 11 \\
Community$_{10}$ & 0.60 & 0.50 & 0.55 & 6 \\
Community$_{11}$ & 0.89 & 0.89 & 0.89 & 9 \\
\hline\hline
accuracy & & & 0.92 & 103 \\
macro avg & 0.92 & 0.88 & 0.88 & 103 \\
weighted avg & 0.92 & 0.92 & 0.91 & 103 \\
\hline
\end{tabular}
\caption{Model Performance on the American College football dataset}
\label{tab:football_PRF}
}
\hfill
\parbox{.5\linewidth}{
\parbox{\linewidth}{
\centering
\begin{tabular}{|c|c|c|c|c|}
\hline
 & precision & recall & f1-score & support \\
\hline\hline
liberal & 0.91 & 1.00 & 0.95 & 42  \\
conservative & 0.88 & 0.96 & 0.92 & 48 \\
neutral & 0.50 & 0.17 & 0.25 & 12 \\
\hline\hline
accuracy & & & 0.88 & 102 \\
macro avg & 0.77 & 0.71 & 0.71 & 102 \\
weighted avg & 0.85 & 0.88 & 0.86 & 102 \\
\hline
\end{tabular}
\caption{Model Performance on the Books about US politics dataset\\}
\label{tab:polbooks_PRF}
}
\parbox{\linewidth}{
\centering
\begin{tabular}{|c|c|c|c|c|}
\hline
 & precision & recall & f1-score & support \\ [0.5ex]
\hline\hline
pos. edge & 0.88 & 0.93 & 0.90 & 15,620  \\
neg. edge & 0.93 & 0.87 & 0.90 & 15,620 \\
\hline\hline
accuracy & & & 0.90 & 31,240 \\
macro avg & 0.90 & 0.90 & 0.90 & 31,240 \\
weighted avg & 0.90 & 0.90 & 0.90 & 31,240 \\ [0.5ex]
\hline
\end{tabular}
\caption{Model Performance on the PPI dataset}
\label{tab:PPI_PRF}
}}
\end{table}
\begin{table}[H]
\setlength{\tabcolsep}{5pt}
\parbox{.5\linewidth}{
\centering
\begin{tabular}{|c|c|c|c|c|}
\hline
 & precision & recall & f1-score & support \\ [0.5ex]
\hline\hline
pos. edge & 0.75 & 0.84 & 0.79 & 25,000  \\
neg. edge & 0.81 & 0.72 & 0.76 & 25,000 \\
\hline\hline
accuracy & & & 0.78 & 50,000 \\
macro avg & 0.78 & 0.78 & 0.77 & 50,000 \\
weighted avg & 0.78 & 0.78 & 0.77 & 50,000 \\ [0.5ex]
\hline
\end{tabular}
\caption{Model Performance on the DDI dataset}
\label{tab:DDI_PRF}
}
\hfill
\parbox{.5\linewidth}{
\centering
\begin{tabular}{|c|c|c|c|c|}
\hline
 & precision & recall & f1-score & support \\ [0.5ex]
\hline\hline
pos. edge & 0.77 & 0.96 & 0.86 & 4,500  \\
neg. edge & 0.95 & 0.72 & 0.82 & 4,500 \\
\hline\hline
accuracy & & & 0.84 & 9,000 \\
macro avg & 0.86 & 0.84 & 0.84 & 9,000 \\
weighted avg & 0.86 & 0.84 & 0.84 & 9,000 \\ [0.5ex]
\hline
\end{tabular}
\caption{Model Performance on the DTI dataset}
\label{tab:DTI_PRF}
}
\end{table}
